# Supplementary material for: Vecchia-Laplace approximations of generalized Gaussian processes for big non-Gaussian spatial data
Source: arXiv:1906.07828 ancillary file (2020-06-04)
Supplement: Supplementary file 1 [file vecchia_laplace_supp.pdf]

# Vecchia-Laplace approximations of generalized Gaussian processes for big non-Gaussian spatial data: Supplementary material

Daniel Zilber[*] Matthias Katzfuss[*†]

June 21, 2019

## S1 Vecchia-Laplace likelihood

We follow the approach of Katzfuss and Guinness (2017), replacing the Gaussian observation $\mathbf{z}$ with the pseudo-observation $\mathbf{t}$ and extending to the case $\boldsymbol{\mu} \neq \mathbf{0}$. Note first that $p(\mathbf{x})/p(\mathbf{y}|\mathbf{t}) = p(\mathbf{t})$. From Section 2.3, the density of $\mathbf{x}$ resulting from general Vecchia has the form $p(\mathbf{x}) = \mathcal{N}(\boldsymbol{\mu}_x, \mathbf{Q}^{-1})$. The denominator is given by the posterior and has the form $p(\mathbf{y}|\mathbf{t}) = \mathcal{N}(\boldsymbol{\alpha}, \mathbf{W}_{\boldsymbol{\alpha}}^{-1})$. Thus,

$$\begin{aligned}\log p(\mathbf{t}) = &-\frac{1}{2}(\mathbf{x}-\boldsymbol{\mu}_x)'\mathbf{Q}(\mathbf{x}-\boldsymbol{\mu}_x) + \frac{1}{2}\log|\mathbf{Q}| - \frac{2n}{2}\log(2\pi)\\ &+\frac{1}{2}(\mathbf{y}-\boldsymbol{\alpha})'\mathbf{W}_{\boldsymbol{\alpha}}(\mathbf{y}-\boldsymbol{\alpha}) - \frac{1}{2}\log|\mathbf{W}_{\boldsymbol{\alpha}}| + \frac{n}{2}\log(2\pi)\end{aligned}$$

By definition $\mathbf{Q} = \mathbf{U}\mathbf{U}'$, so the determinant simplifies according to $\log|\mathbf{Q}| = 2\log|\mathbf{U}|$. Similarly, $\mathbf{W} = \mathbf{U}_y\mathbf{U}_y' = \mathbf{V}\mathbf{V}'$, where $\mathbf{V} = \text{chol}(\mathbf{W})$, so $\log|\mathbf{W}| = 2\log|\mathbf{V}|$. Expanding the term $(\mathbf{x} - \boldsymbol{\mu}_x)'\mathbf{Q}(\mathbf{x}-\boldsymbol{\mu}_x)$ yields:

$$\begin{aligned}(\mathbf{x}-\boldsymbol{\mu}_x)'\mathbf{Q}(\mathbf{x}-\boldsymbol{\mu}_x) &= \begin{bmatrix}\mathbf{y}-\boldsymbol{\mu}, & \mathbf{t}-\boldsymbol{\mu}_t\end{bmatrix}\begin{bmatrix}\mathbf{U}_y\mathbf{U}_y' & \mathbf{U}_y\mathbf{U}_t' \\ \mathbf{U}_t\mathbf{U}_y' & \mathbf{U}_t\mathbf{U}_t'\end{bmatrix}\begin{bmatrix}\mathbf{y}-\boldsymbol{\mu} \\ \mathbf{t}-\boldsymbol{\mu}_t\end{bmatrix}\\ &= (\mathbf{y}-\boldsymbol{\mu})'\mathbf{W}(\mathbf{y}-\boldsymbol{\mu}) + (\mathbf{t}-\boldsymbol{\mu}_t)'\mathbf{U}_t\mathbf{U}_t'(\mathbf{t}-\boldsymbol{\mu}_t) + 2(\mathbf{y}-\boldsymbol{\mu})'\mathbf{U}_y\mathbf{U}_t'(\mathbf{t}-\boldsymbol{\mu}_t),\end{aligned}$$

where $\boldsymbol{\mu}_t = \text{E}(\mathbf{y}) + \mathbf{0} = \boldsymbol{\mu}$ according to our model for the pseudo-data. Subtracting the term $\mathbf{y}'\mathbf{W}\mathbf{y}$ that occurs in the denominator and plugging in for $\mathbf{y}$ the mode found via Vecchia-Laplace

[*]Department of Statistics, Texas A&M University
[†]Corresponding author: katzfuss@gmail.com

iterations, $\boldsymbol{\alpha} = \boldsymbol{\mu} - \mathbf{W}^{-1}\mathbf{U}_y\mathbf{U}_t'(\mathbf{t} - \boldsymbol{\mu})$, we are left with

$$\begin{aligned}
\log p(\mathbf{t}) =& -\frac{1}{2}(\mathbf{t} - \boldsymbol{\mu}_t)'\mathbf{U}_t\mathbf{U}_t'(\mathbf{t} - \boldsymbol{\mu}) - (\mathbf{y} - \boldsymbol{\mu})'\mathbf{U}_y\mathbf{U}_t'(\mathbf{t} - \boldsymbol{\mu}) - \frac{1}{2}\boldsymbol{\mu}'\mathbf{W}\boldsymbol{\mu} \\
& + \mathbf{y}'\big[\mathbf{W}\boldsymbol{\mu} - \mathbf{W}(\boldsymbol{\mu} - \mathbf{W}^{-1}\mathbf{U}_y\mathbf{U}_t'(\mathbf{t} - \boldsymbol{\mu}))\big] - \frac{n}{2}\log(2\pi) + \log|\mathbf{U}| - \log|\mathbf{V}| \\
& + \frac{1}{2}(\boldsymbol{\mu} - \mathbf{W}^{-1}\mathbf{U}_y\mathbf{U}_t'(\mathbf{t} - \boldsymbol{\mu}))'\mathbf{W}(\boldsymbol{\mu} - \mathbf{W}^{-1}\mathbf{U}_y\mathbf{U}_t'(\mathbf{t} - \boldsymbol{\mu})) \\
=& -\frac{1}{2}(\mathbf{t} - \boldsymbol{\mu})'\mathbf{U}_t\mathbf{U}_t'(\mathbf{t} - \boldsymbol{\mu}) + \frac{1}{2}(\mathbf{t} - \boldsymbol{\mu})\mathbf{U}_t\mathbf{U}_y'\mathbf{W}^{-1}\mathbf{U}_y\mathbf{U}_t'(\mathbf{t} - \boldsymbol{\mu}) - (\mathbf{y} - \boldsymbol{\mu})'\mathbf{U}_y\mathbf{U}_t'(\mathbf{t} - \boldsymbol{\mu}) \\
& + \frac{1}{2}\boldsymbol{\mu}'\mathbf{W}\boldsymbol{\mu} - \frac{1}{2}\boldsymbol{\mu}'\mathbf{W}\boldsymbol{\mu} + \mathbf{y}'\big[\mathbf{U}_y\mathbf{U}_t'(\mathbf{t} - \boldsymbol{\mu})\big] - \boldsymbol{\mu}\mathbf{U}_y\mathbf{U}_t'(\mathbf{t} - \boldsymbol{\mu}) \\
& - \frac{n}{2}\log(2\pi) + \log|\mathbf{U}| - \log|\mathbf{V}| \\
=& -\frac{1}{2}(\mathbf{t} - \boldsymbol{\mu})'(\mathbf{U}_t\mathbf{U}_t' - \mathbf{U}_t\mathbf{U}_y'\mathbf{W}^{-1}\mathbf{U}_y\mathbf{U}_t')(\mathbf{t} - \boldsymbol{\mu}) - \frac{n}{2}\log(2\pi) + \log|\mathbf{U}| - \log|\mathbf{V}| \\
& + (\mathbf{y}' - \boldsymbol{\mu})\mathbf{U}_y\mathbf{U}_t'(\mathbf{t} - \boldsymbol{\mu}) - (\mathbf{y} - \boldsymbol{\mu})'\mathbf{U}_y\mathbf{U}_t'(\mathbf{t} - \boldsymbol{\mu}) \\
=& -\frac{n}{2}\log(2\pi) + \log|\mathbf{U}| - \log|\mathbf{V}| \\
& - \frac{1}{2}(\mathbf{t} - \boldsymbol{\mu})'\mathbf{U}_t\mathbf{U}_t'(\mathbf{t} - \boldsymbol{\mu}) + \frac{1}{2}(\mathbf{t} - \boldsymbol{\mu})'\mathbf{U}_t\mathbf{U}_y'\mathbf{W}^{-1}\mathbf{U}_y\mathbf{U}_t'(\mathbf{t} - \boldsymbol{\mu}).
\end{aligned}$$

# S2 Extended algorithmic example

Algorithm 2 provides pseudo-code for VL prediction and parameter estimation.

# S3 Details for comparison to Hamiltonian Monte Carlo (HMC)

## S3.1 HMC results

As described in Section 4.1, we simulated a single dataset consisting of $n = 625$ Bernoulli observations with $\nu = .5$, and compared Laplace and VL methods with $m = 10$ to HMC with path step size of $\epsilon = .001$ and a path step count (leapfrog iteration count) of $L = 50$. We ran HMC for 300,000 iterations to get an estimate for the true posterior. To account for finite computing resources and have a fair comparison to VL, we also ran HMC for 8,000 iterations and repeated this 20 times to average out randomness. For all HMC runs, we used a burn-in of 5,000 iterations and thinned the remaining samples by a factor of 10.

| Method | Iterations ($k$) | Complexity | RMSE | Time (s) |
|---|---|---|---|---|
| HMC | 300,000 | $\mathcal{O}(k(Ln + n^3))$ | 0.634 | 6928.4 |
| HMC | 8,000 | $\mathcal{O}(k(Ln + n^3))$ | 0.929 | 276.8 |
| Laplace | <10 | $\mathcal{O}(kn^3)$ | 0.639 | 1.2 |
| VL-DL | <10 | $\mathcal{O}(kn)$ | 0.639 | 0.1 |

Table S1: Comparison to HMC for $n = 625$ simulated Bernoulli data

The comparison results are shown in Table S1. Timings were acquired on a laptop, and the RRMSE is only based on a single simulated dataset, so the table can only serve as a rough comparison. While HMC typically exhibits better mixing than Metropolis-Hastings sampling, HMC with $k = 8{,}000$ iterations was less accurate than Laplace-based methods despite being several orders of

**Algorithm 2** VL Prediction and Parameter Estimation

**procedure** PARAMETER ESTIMATION($\mathbf{z}, \mathcal{S}, g$)
    Define and initialize parameter vector, e.g., $\boldsymbol{\theta} = (\boldsymbol{\mu}', \nu, \rho, \sigma^2)'$
    Run VECCHIA-SPECIFY($\mathcal{S}, m$) with VL-IW to obtain $\texttt{VAO}_2$
    **if** dim = 1 **then**
        Set $\texttt{VAO}_1 = \texttt{VAO}_2$
    **else**
        Run VECCHIA-SPECIFY($\mathcal{S}, m$) with VL-RF to obtain $\texttt{VAO}_1$
    **end if**
    **repeat**
        Obtain new value of $\theta$ (e.g., using Nelder-Mead)
        Run VL-LIKELIHOOD($\mathbf{z}, \mathcal{S}, \texttt{VAO}_1, \texttt{VAO}_2, g, \boldsymbol{\mu}, K_{\boldsymbol{\theta}}$) to get $\mathcal{L}_{VL}(\boldsymbol{\theta})$
    **until** convergence
    **return** $\hat{\boldsymbol{\theta}} = \boldsymbol{\theta}$
**end procedure**

**procedure** VL-LIKELIHOOD($\mathbf{z}, \mathcal{S}, \texttt{VAO}_1, \texttt{VAO}_2, g, \boldsymbol{\mu}, K$)
    Run VL-INFERENCE using $\texttt{VAO}_1$ to obtain the posterior mode $\boldsymbol{\alpha}_V$ and pseudo-data $\mathbf{t}, \mathbf{D}$
    Evaluate $\mathcal{L}_{VL}(\boldsymbol{\theta})$ in Eqt. (10) using the data, $\boldsymbol{\theta}, \mathbf{t}, \mathbf{D}$, based on $\texttt{VAO}_2$
    **return** $\mathcal{L}_{VL}(\boldsymbol{\theta})$
**end procedure**

**procedure** VL-PREDICTION( $\mathbf{z}, \mathcal{S}, \mathcal{S}^\star, g, \boldsymbol{\theta}$)
    Run VECCHIA-SPECIFY($\mathcal{S}, m, \mathcal{S}^\star$) to get $\texttt{VAO}$ (Use VL-RF if dim $> 1$)
    Run VL-INFERENCE with $\texttt{VAO}$ to obtain the posterior mode $\boldsymbol{\alpha}_V$ and pseudo-data $\mathbf{t}, \mathbf{D}$
    Perform latent prediction (Section 3.4) with $\boldsymbol{\alpha}_V, \mathbf{t}, \mathbf{D}$ to get $(\mathbf{y}^\star, \mathbf{y})|\mathbf{t} \sim N(\widetilde{\boldsymbol{\mu}}, (\widetilde{\mathbf{V}}\widetilde{\mathbf{V}}')^{-1})$
    If desired, obtain predictive summaries of $\mathbf{z}^\star$ by transforming samples of $\mathbf{y}^\star$ based on $g(z|y)$
    **return** Predictions and uncertainty measures of $\mathbf{y}^\star$ (and $\mathbf{z}^\star$)
**end procedure**

magnitude slower. For larger $n$, the performance of HMC will likely degrade even further relative to VL, due to its cubic scaling in $n$ for each iteration, and the increased number of required iterations for convergence.

### S3.2 HMC trace plots

Figure S1 shows a set of the trace plots that result from running Hamiltonian Monte Carlo (HMC). The plots show the path taken by the variable in the specified position, so that the first plot shows 10th latent variable, etc. HMC was run for 300,000 iterations with a burn-in of 5,000 and a 10:1 thinning applied to the remaining values.

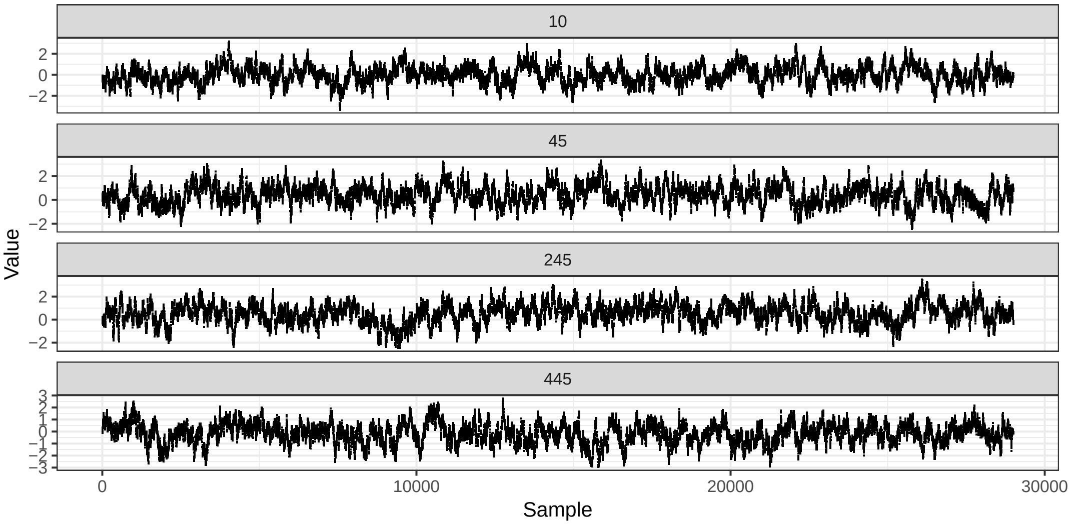


Figure S1: Trace plot showing sample paths for four latent variables for Hamiltonian Monte Carlo

## S4 Higher-dimensional simulations

While we have focused on one- and two-dimensional space, we also briefly examined the performance of VL in three and four dimensions using simulation. In Figures S2 and S3 below, the sample size was $13^3 = 2197$ and $7^4 = 2401$ for the 3D and 4D demonstrations. Due to the relatively small number of points per axis, the range parameters were increased to $\rho_{3D} = .1$ and $\rho_{4D} = .2$. The relative performance between VL and LowRank was quite similar to the 2D scenario, and we expect this to hold in higher dimensions as well.

## S5 Qualitative comparison of predictions in 1-D

Here we present a few qualitative advantages of VL over LowRank. Figure S4a demonstrates the visual difference between the approximations we compared. While the VL approximation was similar to the Laplace approximation, the low-rank approximation exhibited spikes that correspond to the correction terms of the modified predictive process. As a prediction location became far from the knots, the correction term increased up to the process variance at the location and resulted in artifacts, as shown in Figure S4c.

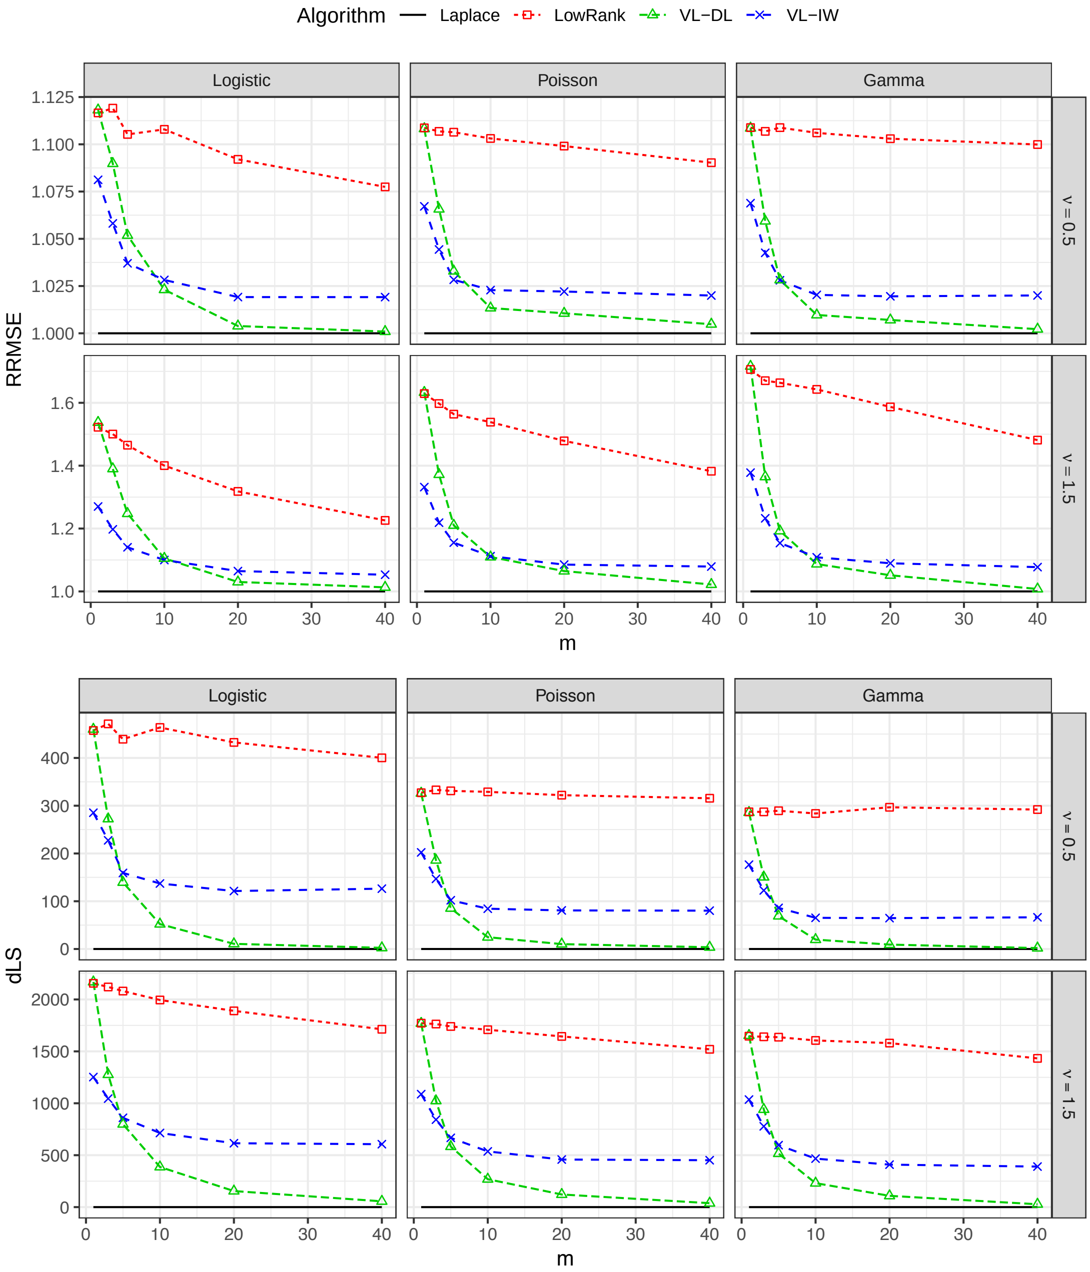


Figure S2: Relative root mean square error (RRMSE) and Log Score difference from Laplace (dLS) for **3D** data

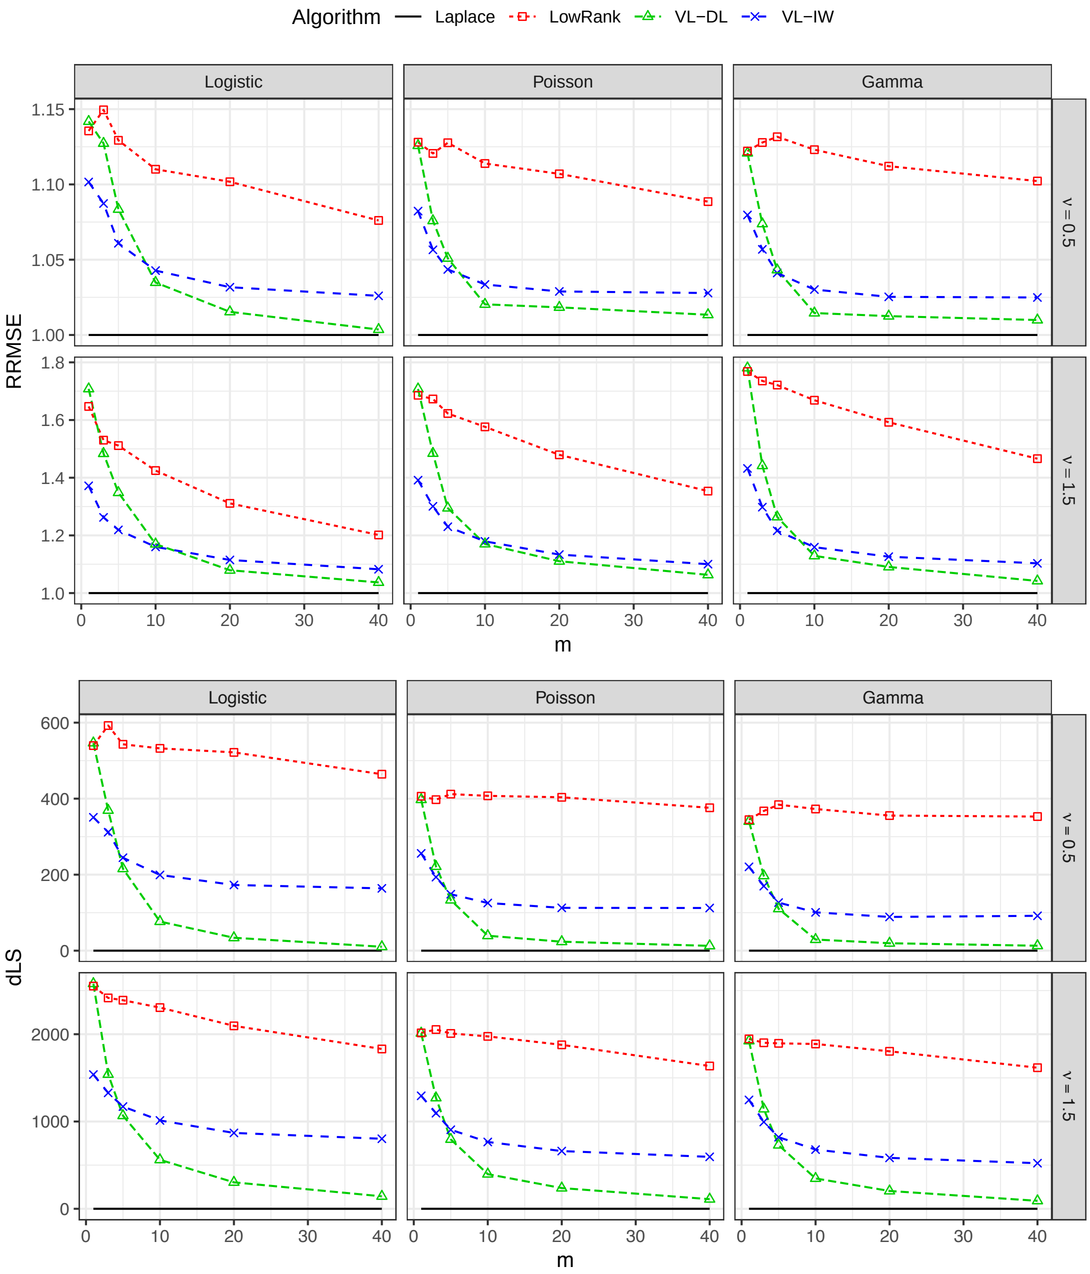


Figure S3: Relative root mean square error (RRMSE) and Log Score difference from Laplace (dLS) for **4D** data

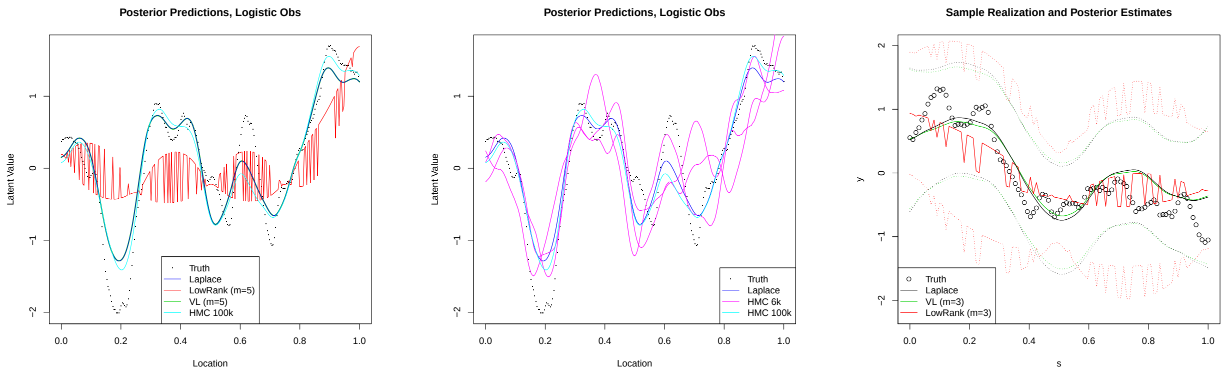


(a) Summary comparison (b) HMC (c) MPP showing correction terms

Figure S4: Comparison plots showing the posterior estimates of various methods

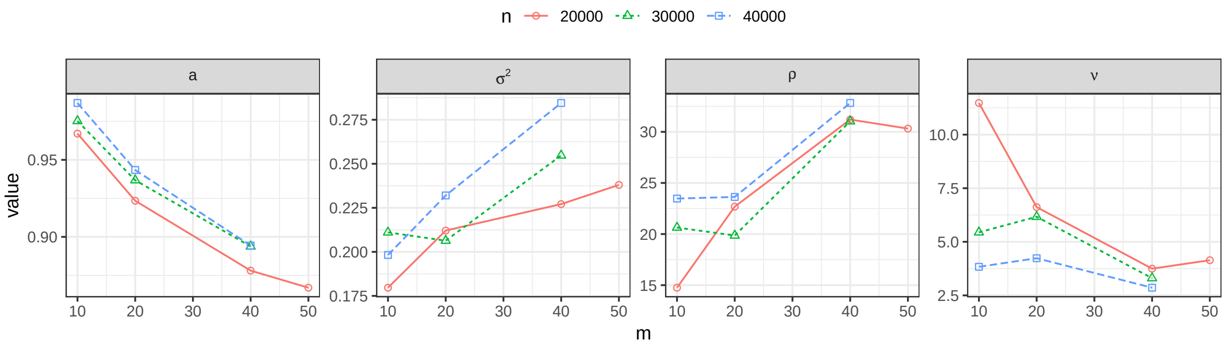


Figure S5: Results of exploratory parameter estimation for the shape parameter $a$ and covariance parameters $(\sigma^2, \rho, \nu)$ for variance, range, and smoothness. We concluded that $a = .89$, $\sigma^2 = .25$, $\rho = 31$km, and $\nu = 3$ were reasonable values.

# S6 Parameter estimation for MODIS data

To apply the spatial Gamma GGP model described in Section 5, we needed to estimate several parameters: the Gamma shape parameter $a$, the trend parameter $\boldsymbol{\beta} = (\beta_1, \beta_2)'$, and the Matérn covariance parameters $\boldsymbol{\theta} = (\sigma^2, \rho, \nu)'$ determining the variance, range and smoothness. Simply estimating all parameters together based on the integrated likelihood was not possible due to identifiability issues.

Our parameter estimation procedure began by estimating the linear trend parameter $\boldsymbol{\beta}$. We temporarily ignored dependence in the residuals and essentially assumed a generalized linear model (McCullagh and Nelder, 1989). Thus, $\boldsymbol{\beta}$ was fitted with the standard technique of iteratively reweighted least squares using a subsample of 1,000,000 data points, yielding the estimated value $\boldsymbol{\beta} = (-1.515, 0.000766)'$.

Then, given $\boldsymbol{\beta}$, we carried out an iterative procedure in which we alternated between optimizing the covariance parameters $\boldsymbol{\theta}$ conditional on the shape parameter $a$, and vice versa. The covariance parameters $\boldsymbol{\theta}$ were obtained by maximizing the integrated VL likelihood from Section 3.3 via the Nelder-Mead algorithm, as described by Algorithm 2 in Section S2. The shape parameter $a$ was estimated by maximizing $p(\mathbf{z}|\mathbf{y} = \boldsymbol{\alpha}_V)$ with $\boldsymbol{\alpha}_V$ obtained using the VL Algorithm 1 based on $\boldsymbol{\beta}$ and the current estimate of $\boldsymbol{\theta}$. We believe that this approach can result in more accurate estimates of $a$ relative to estimates obtained under the assumption of $\mathbf{y} = \boldsymbol{\mu}$ (e.g. Sengupta and Cressie, 2013).

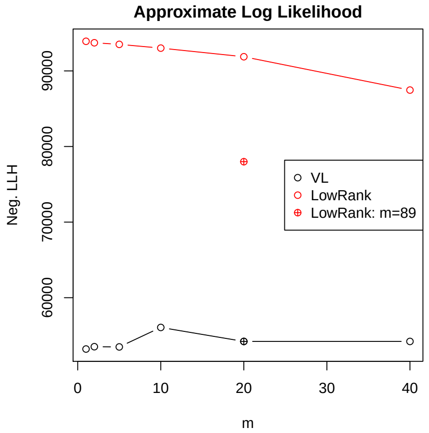


Figure S6: The integrated VL likelihood was virtually constant between $m = 20$ and $m = 40$, while the LowRank likelihood varied greatly in comparison. The crossed points compare the likelihoods for the $m$ values used in the application in Section 5.

While we found that three iterations of alternating between estimating $\boldsymbol{\theta}$ and $a$ typically sufficed for convergence, in total this procedure still required hundreds of calls to the VL Algorithm 1, which could be quite time-consuming for large sample sizes. Hence, as shown in Figure S5, we progressively increased the (subsampled) sample size $n$ from 10,000 to 40,000 and conditioning set size $m$ from 10 to 50 until the estimates started to converge. While the individual parameter estimates changed slightly as a function of $m$, Figure S6 shows that the integrated VL likelihood for fixed $n = 250,000$ was virtually identical between $m = 20$ and $m = 40$. The integrated likelihood implied by LowRank was considerably worse.

Together, these results led us to conclude that $a = 0.89, \sigma^2 = .25, \rho = 31, \nu = 3$ were reasonable parameter values, and that $m = 20$ was adequate for VL in the prediction comparisons shown in Section 5.

# References

Katzfuss, M. and Guinness, J. (2017). A general framework for Vecchia approximations of Gaussian processes. *arXiv:1708.06302*.

McCullagh, P. and Nelder, J. A. (1989). *Generalized Linear Models*. CRC press.

Sengupta, A. and Cressie, N. (2013). Hierarchical statistical modeling of big spatial datasets using the exponential family of distributions. *Spatial Statistics*, 4:14–44.
